# Supplementary material for: Evaluating the Values of Sources in Transfer Learning
Source: arXiv:2104.12567 source file (2021-04-26)
Supplement: Supplementary file 1 [file main-appendix.tex]

%
% File emnlp2020.tex
%
%% Based on the style files for ACL 2020, which were
%% Based on the style files for ACL 2018, NAACL 2018/19, which were
%% Based on the style files for ACL-2015, with some improvements
%%  taken from the NAACL-2016 style
%% Based on the style files for ACL-2014, which were, in turn,
%% based on ACL-2013, ACL-2012, ACL-2011, ACL-2010, ACL-IJCNLP-2009,
%% EACL-2009, IJCNLP-2008...
%% Based on the style files for EACL 2006 by 
%%e.agirre@ehu.es or Sergi.Balari@uab.es
%% and that of ACL 08 by Joakim Nivre and Noah Smith

\documentclass[11pt]{article}
\usepackage[review]{naacl2021}
\usepackage{times}
\usepackage{latexsym}

\usepackage{multirow}
% This is not strictly necessary, and may be commented out,
% but it will improve the layout of the manuscript,
% and will typically save some space.
\usepackage{microtype}
\usepackage{booktabs}
\usepackage{graphicx}
\usepackage[ruled,linesnumbered]{algorithm2e}
\usepackage{enumitem}
\usepackage{subfigure}
\usepackage{paralist}

\usepackage{longtable}
\usepackage{makecell}

\usepackage{url}
\usepackage{comment}
\usepackage[flushleft]{threeparttable}

\usepackage{amsmath}

\usepackage{tabularx}

\usepackage{todonotes}

\linespread{1.0}

\aclfinalcopy

%\aclfinalcopy % Uncomment this line for the final submission
%\def\aclpaperid{***} %  Enter the acl Paper ID here

%\setlength\titlebox{5cm}
% You can expand the titlebox if you need extra space
% to show all the authors. Please do not make the titlebox
% smaller than 5cm (the original size); we will check this
% in the camera-ready version and ask you to change it back.

\title{Choosing Transfer Sources using Approximated Shapley Values}

\author{First Author \\
  Affiliation / Address line 1 \\
  Affiliation / Address line 2 \\
  Affiliation / Address line 3 \\
  \texttt{email@domain} \\\And
  Second Author \\
  Affiliation / Address line 1 \\
  Affiliation / Address line 2 \\
  Affiliation / Address line 3 \\
  \texttt{email@domain} \\}

\date{}

\begin{document}

\cleardoublepage
\input{appendix}

\bibliography{emnlp2020}
\bibliographystyle{acl_natbib}

\end{document}
